# Supplementary material for: SoK: Yield Aggregators in DeFi
Source: arXiv:2105.13891 source file (2022-03-27)
Supplement: Supplementary file 1 [file appendices.tex]

\newpage
